# Supplementary material for: Mitigation of Measurement-Induced State Transitions via a Fast-Load and Fast-Clear Readout
Source: arXiv:2607.23681 source file (2026-07-26)
Supplement: Supplementary file 1 [file SM.tex]

% ****** Start of file apssamp.tex ******
%
%   This file is part of the APS files in the REVTeX 4.2 distribution.
%   Version 4.2a of REVTeX, December 2014
%
%   Copyright (c) 2014 The American Physical Society.
%
%   See the REVTeX 4 README file for restrictions and more information.
%
% TeX'ing this file requires that you have AMS-LaTeX 2.0 installed
% as well as the rest of the prerequisites for REVTeX 4.2
%
% See the REVTeX 4 README file
% It also requires running BibTeX. The commands are as follows:
%
%  1)  latex apssamp.tex
%  2)  bibtex apssamp
%  3)  latex apssamp.tex
%  4)  latex apssamp.tex
%
\documentclass[%
 reprint,
 aps,
 prapplied,
 amsmath,amssymb,
 superscriptaddress,
 floatfix,
]{revtex4-2}
\usepackage{hyperref}% add hypertext capabilities
\hypersetup{colorlinks=true,linkcolor=blue,citecolor=blue}
\usepackage[caption=false]{subfig}
\usepackage{graphicx}% Include figure files
\usepackage{dcolumn}% Align table columns on decimal point
\usepackage{bm}% bold math
\usepackage[caption=false]{subfig}
\usepackage{booktabs}
%\usepackage[mathlines]{lineno}% Enable numbering of text and display math
%\linenumbers\relax % Commence numbering lines

%\usepackage[showframe,%Uncomment any one of the following lines to test 
%%scale=0.7, marginratio={1:1, 2:3}, ignoreall,% default settings
%%text={7in,10in},centering,
%%margin=1.5in,
%%total={6.5in,8.75in}, top=1.2in, left=0.9in, includefoot,
%%height=10in,a5paper,hmargin={3cm,0.8in},
%]{geometry}

\begin{document}
\renewcommand{\thefigure}{S\arabic{figure}}
\setcounter{figure}{0}
\renewcommand{\theequation}{S\arabic{equation}}
\setcounter{equation}{0}

\preprint{APS/123-QED}

\title{Supplementary Material for “Mitigation of Measurement-Induced State Transitions via a Fast-Load and Fast-Clear Readout”}% Force line breaks with \\

\author{Wei-En Lin}
\thanks{These two authors contributed equally to this work.} 
\affiliation{Research Center for Critical Issues, Academia Sinica, Tainan, 711010, Taiwan}
\affiliation{Department of Physics, National Central University, Taoyuan, 320317, Taiwan}

\author{Li-Chieh Hsiao}
\thanks{These two authors contributed equally to this work.}
\affiliation{Research Center for Critical Issues, Academia Sinica, Tainan, 711010, Taiwan}
\affiliation{Department of Physics, National Cheng Kung University, Tainan, 701401, Taiwan}

\author{Chen-Hsun Ma}
\affiliation{Research Center for Critical Issues, Academia Sinica, Tainan, 711010, Taiwan}
\affiliation{Department of Physics, National Taiwan University, Taipei, 106319, Taiwan}

\author{Erh-Hsiang Yeh}
\affiliation{Department of Physics, National Central University, Taoyuan, 320317, Taiwan}

\author{Wei-Lun Peng}
\affiliation{Department of Physics, National Changhua University of Education, Changhua, 500207, Taiwan}

\author{Hsi-Sheng Goan}
\affiliation{Department of Physics, National Taiwan University, Taipei, 106319, Taiwan}
\affiliation{Center for Quantum Science and Engineering, National Taiwan University, Taipei, 106319, Taiwan}
\affiliation{Physics Division, National Center for Theoretical Sciences, Taipei, 106319, Taiwan}

\author{Cen-Shawn Wu}
\affiliation{Research Center for Critical Issues, Academia Sinica, Tainan, 711010, Taiwan}
\affiliation{Department of Physics, National Changhua University of Education, Changhua, 500207, Taiwan}

\author{Yueh-Nan Chen}
\affiliation{Department of Physics, National Cheng Kung University, Tainan, 701401, Taiwan}
\affiliation{Physics Division, National Center for Theoretical Sciences, Taipei, 106319, Taiwan}
\affiliation{Center for Quantum Frontiers of Research and Technology, National Cheng Kung University, Tainan, 701401, Taiwan}

\author{Yung-Fu Chen}\email{yfuchen@cc.ncu.edu.tw}
\affiliation{Department of Physics, National Central University, Taoyuan, 320317, Taiwan}
\affiliation{Center of High Energy and High Field Physics, National Central University, Taoyuan, 320317, Taiwan}
\affiliation{Quantum Technology Center, National Central University, Taoyuan, 320317, Taiwan}
\affiliation{Taiwan Semiconductor Research Institute, National Institutes of Applied Research, Hsinchu, 300091, Taiwan}
\affiliation{National Center for Excellence in Quantum Information Science and Engineering, National Tsing Hua University, Hsinchu, 300044, Taiwan }

\author{Chung-Ting Ke}\email{ctke@gate.sinica.edu.tw}
\affiliation{Research Center for Critical Issues, Academia Sinica, Tainan, 711010, Taiwan}
\affiliation{Institute of Physics, Academia Sinica, Taipei, 115201, Taiwan}

\author{Chii-Dong Chen}
\affiliation{Research Center for Critical Issues, Academia Sinica, Tainan, 711010, Taiwan}
\affiliation{Institute of Physics, Academia Sinica, Taipei, 115201, Taiwan}

\maketitle
\onecolumngrid

\addtocontents{toc}{\protect\setcounter{tocdepth}{2}} 
\tableofcontents 
\newpage

\begin{figure*}  
\centering
\includegraphics[width=\textwidth]{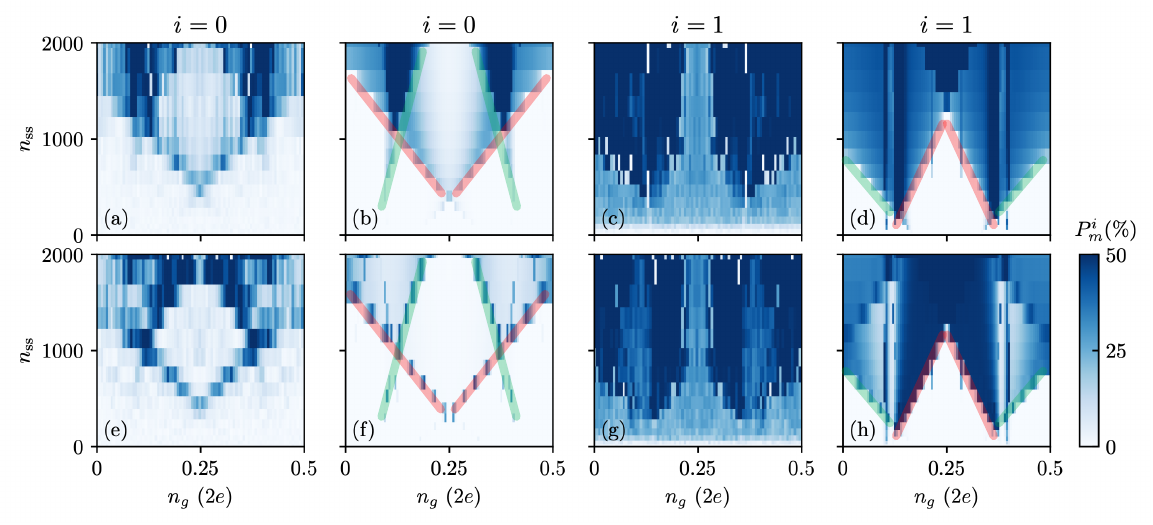} 
\caption{MIST structures of qubit Q2 associated with $M_2$ and their suppression via pulse shaping for initial qubit states $|i\rangle$. MIST structures versus $n_g$ and $n_{\text{ss}}$, characterized by $P^i_m$, are shown for a square pulse in (a),(c) as measured and (b),(d) as simulated, with the experimental data benchmarked against the numerical simulations. The suppression of MIST features achieved via a two-step pulse scheme is shown in (e),(g) as measured and (f),(h) as simulated. The red and green semi-transparent guide lines overlaying (b),(f) apply to the qubit prepared in $\vert0\rangle$, tracing the transitions from $B_0$ to branches $B_6$ and $B_8$, respectively. The same color sequence in (d),(h) applies to the qubit prepared in $\vert1\rangle$, tracing the transitions from $B_1$ to branches $B_5$ and $B_7$. }
\label{S1}
\end{figure*}

\section{Mitigation of MIST during readout for Q2}
\label{S:sec:during}

We present measurements on qubit Q2 together with the corresponding numerical simulations, mapping out the measurement-induced state transition (MIST) structure as a function of the offset charge $n_g$ and the steady-state photon number $n_{\text{ss}}$, following the protocol of Fig.~2(c) in the main text. For the $M_2$ pulse, we employ $4\,\mu\text{s}$ waveforms with square, two-step, and three-step profiles. The two-step and three-step profiles use a state-independent treatment with $\tau_\uparrow = 100\,\text{ns}$ and $\tau_\uparrow + \tau_{\text{ss}} = 4\,\mu\text{s}$; for the three-step pulse, the ring-down duration is set to $\tau_\downarrow = 100\,\text{ns}$. Both are realized as piecewise-constant pulses: the two-step pulse implements a fast-load scheme, consisting of an initial ring-up stage with parameters $\{\varepsilon_\uparrow, \tau_\uparrow\}$ followed by a steady-state (ss) stage with $\{\varepsilon_{\text{ss}}, \tau_{\text{ss}}\}$, while the three-step pulse additionally implements a fast-clear scheme through an active ring-down segment $\{\varepsilon_\downarrow, \tau_\downarrow\}$ that accelerates the depletion of resonator photons. Here $\varepsilon$ and $\tau$ denote the drive amplitude and duration of each segment, respectively. For $M_1$ and $M_3$, we apply weak square pulses of $8\,\mu\text{s}$ duration, with an $8\,\mu\text{s}$ idle time between readouts.

In this section, we investigate the mitigation of MIST during readout of Q2, probing the transition probability $P^i_{m}$ with the $M_2$ pulse. Since the three-step pulse differs from the two-step pulse only by its additional ring-down segment, which acts after readout, the two produce identical $M_2$ results. Therefore, we compare only the square and two-step pulses here. Figure~\ref{S1} compares the MIST structure obtained with the square profile in Figs.~\ref{S1}(a)--(d) and the calibrated two-step profile in Figs.~\ref{S1}(e)--(h). In each panel, several bands of elevated transition probability are visible, indicating MIST. To identify their origin, we perform a numerical Floquet branch analysis. The red and green semi-transparent guide lines in Figs.~\ref{S1}(b) and (f) trace the transitions from $B_0$ to $B_6$ and from $B_0$ to $B_8$, respectively, while those in Figs.~\ref{S1}(d) and (h) follow the same color order to trace the transitions from $B_1$ to $B_5$ and from $B_1$ to $B_7$, respectively. The higher background probability primarily arises from decoherence, which was not accounted for in the simulation. However, the unexpectedly high background observed in the prepared $\vert 1\rangle$ state suggests the presence of additional mechanisms. Aside from the labeled transitions, part of the background MIST is suppressed in both the experimental and numerical results.

To quantify the trade-off between readout signal-to-noise ratio (SNR) and MIST, we evaluate the total readout error $P_{\text{err}}^i = \overline{P^i_{m}}(M_2) + \varepsilon_{o}(M_2)$, where $\overline{P^i_{m}}$ is the $n_g$-averaged transition probability and $\varepsilon_{o}$ the overlap error, both extracted directly from the $M_2$ pulse. The results are summarized in Fig.~\ref{S2}, where we exclude the low-SNR regime with $n_{\text{ss}} < 70$ and the strongly hybridized regime with $n_{\text{ss}} > 1000$, in which $P^i_{m}$ cannot be reliably quantified. Throughout the dynamic regime, both experiment and simulation yield a lower $P^i_{\text{err}}$ for the two-step pulse (red curves) than for the square pulse (blue curves), and the experimental results follow the same trend as the simulations. In a few regions, the measured $P^i_{\text{err}}$ for the two-step pulse appears higher in the experiments. However, the simulations show that the difference between the two profiles is small there, so it is obscured by the statistical uncertainty. Overall, the reduced $P^i_{\text{err}}$ shows that the two-step pulse simultaneously improves readout speed and mitigates MIST.

\section{Mitigation of MIST after readout for Q2} 

In this section, we investigate the mitigation of MIST after readout of Q2 by probing $P^i_{m}$ via the $M_3$ pulse. While the $M_2$ results detailed in Sec.~\ref{S:sec:during} are insensitive to the ring-down and therefore identical for the two-step and three-step pulses, the final qubit state reflects the full pulse evolution, ring-down included. It is for this reason that the square, two-step, and three-step profiles can leave the qubit in distinct post-measurement states. Owing to the critical impact of the resonator ring-down, the $M_3$ behavior is the converse of the $M_2$ results in Fig.~\ref{S1}, where the two-step pulse shows lower MIST than the square pulse. Figure~\ref{S3} compares the $M_3$ responses for both experimental and numerical data under the square profile in Figs.~\ref{S3}(a)--(d), the two-step profile in Figs.~\ref{S3}(e)--(h), and the three-step profile in Figs.~\ref{S3}(i)--(l). In both experiment and simulation, the three-step pulse exhibits the lowest MIST across the dynamic range for $\vert 0\rangle$, whereas the square pulse does so for $\vert 1\rangle$. In both cases, the two-step pulse shows the most severe MIST. The higher background probabilities for the prepared $\vert 1\rangle$ state in Figs.~\ref{S3}(c), (g), and (k) stem primarily from the relaxation error accumulated from state preparation through the end of $M_3$. The band structures observed in experiment are in good agreement with those in simulation.

\begin{figure*}
\centering
\includegraphics[width=\textwidth]{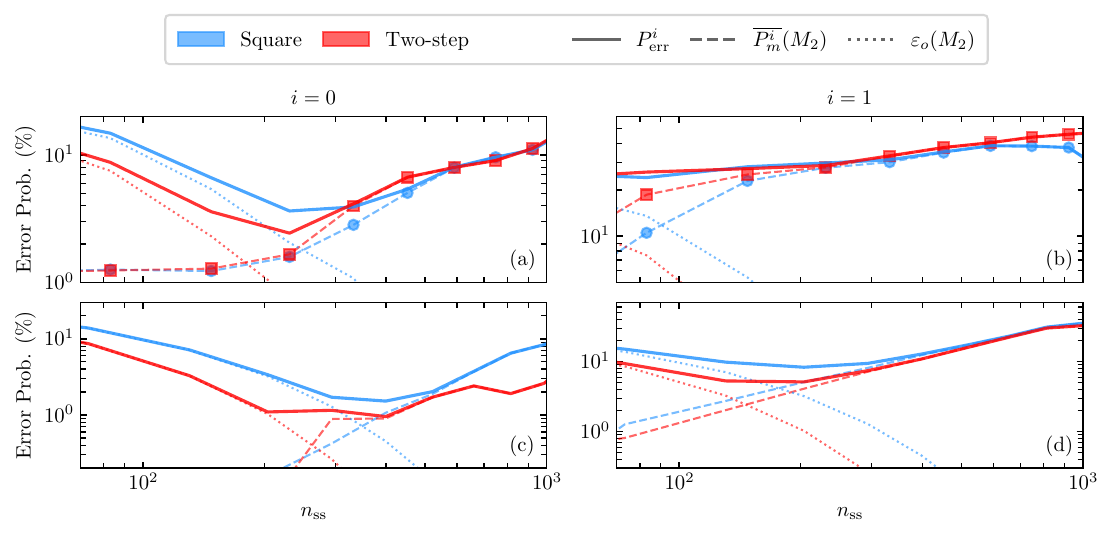} 
\caption{Readout error probabilities for initial qubit states $\vert i\rangle$ as a function of $n_{\mathrm{ss}}$, extracted from the data in Fig.~\ref{S1}. The square and two-step pulses are shown in blue and red, respectively, while solid, dashed, and dotted curves in every panel correspond to the total readout error probability $P_{\mathrm{err}}^i$, the $n_g$-averaged transition probability $\overline{P^i_{m}}(M_2)$, and the overlap error $\varepsilon_{o}(M_2)$, respectively. Experimental data are shown in (a),(b), with the measured $\overline{P^i_{m}}(M_2)$ for the square and two-step pulses marked by dashed curves with circles (blue) and squares (red), respectively. The corresponding numerical simulations are shown in (c),(d).}
\label{S2}
\end{figure*}

\begin{figure*}
\centering
\includegraphics[width=\textwidth]{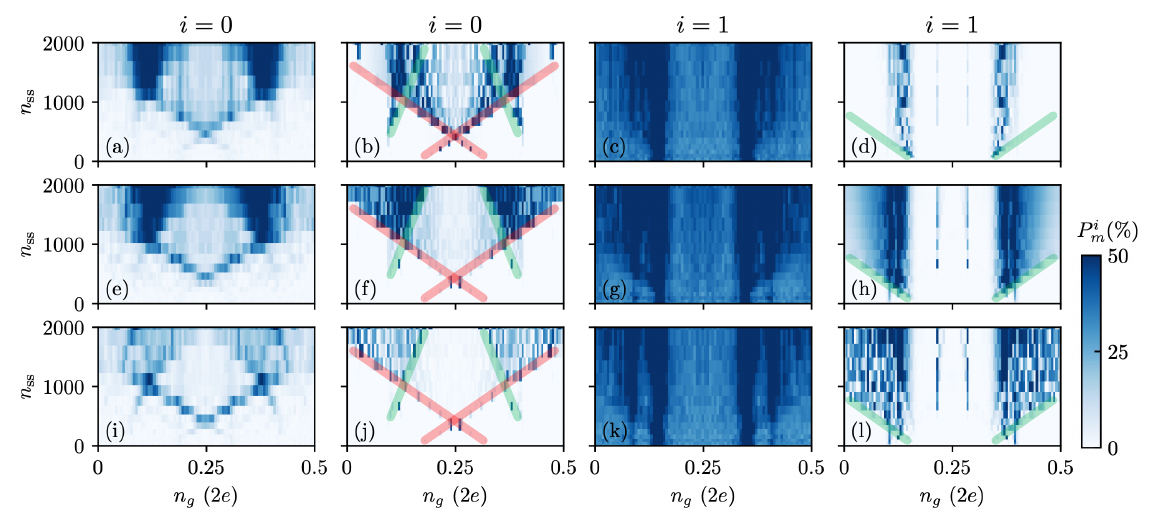} 
\caption{MIST structures of qubit Q2 associated with $M_3$ for initial qubit states $\vert i\rangle$, characterized by $P_{m}^{i}$ as a function of $n_g$ and $n_{\text{ss}}$. Experimental results are grouped by $M_2$ pulse shape, with the square pulse in (a),(c), the two-step pulse in (e),(g), and the three-step pulse in (i),(k), and the corresponding simulations in (b),(d); (f),(h); and (j),(l), respectively. The colored semi-transparent guide lines correspond to the branch transitions defined in Fig.~\ref{S1}.}
\label{S3}
\end{figure*}

Following the same approach, we define the post-readout total error probability as
$\widetilde{P}_{\text{err}}^i = \overline{P^i_{m}}(M_3) + \varepsilon_{o}(M_2)$, comprising the $\overline{P^i_{m}}$ from $M_3$ with the $\varepsilon_{o}$ from $M_2$. For $\vert 0\rangle$, the simulations in Figs.~\ref{S4}(c) and (d) yield a lower $\widetilde{P}_{\text{err}}^i$ for the three-step pulse (green curves) than for the square (blue curves) and two-step (red curves) pulses. For $\vert 1\rangle$, in contrast, the square pulse shows the lowest MIST but the highest $\widetilde{P}_{\text{err}}^i$ in the weakly hybridized regime, as its $\varepsilon_{o}$ outweighs the MIST reduction. In Fig.~\ref{S4}(a), the experimental data follow the same trend as the simulations. In Fig.~\ref{S4}(b), however, the experimental data cannot distinguish the three pulse profiles, owing to the strong background probability seen in Figs.~\ref{S3}(c), (g), and (k). The advantage of the three-step pulse is clearly established for $\vert0\rangle$, where both experiment and simulation give the lowest total error. For $\vert1\rangle$, the advantage is much less pronounced. The reversal between the two initial states can be understood as a competition between diabatic and adiabatic passage through the ionization resonance. For $|0\rangle$, the relevant Landau-Zener gap $\Delta_{\mathrm{ac}}$ is small, so the fast ring-up and ring-down of the three-step pulse traverses the crossing diabatically and conserves the original state, giving the lowest MIST. For $|1\rangle$, in contrast, the gap at the $B_1$ branch crossings is large enough that our ring-up and ring-down rates cannot cross diabatically. The slower ring-up and ring-down of the square pulse then more closely approximates an adiabatic passage, yielding the lowest MIST instead. Overall, the three-step scheme provides the most reliable post-readout state for $|0\rangle$, while for $|1\rangle$ the pulse profiles perform comparably. A faster ring-up and ring-down would likely improve performance further, enabling a more diabatic passage through the $B_1$ crossings and thereby extending the advantage of the three-step scheme to $|1\rangle$.

\begin{figure*}
\centering
\includegraphics[width=\textwidth]{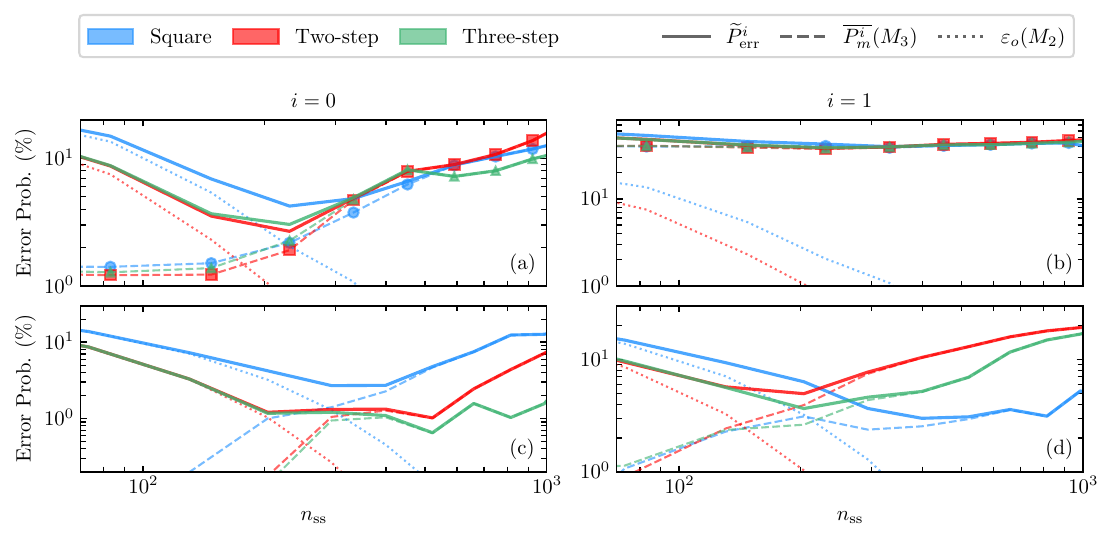} 
\caption{Post-readout error probabilities for initial qubit states $\vert i\rangle$ as a function of $n_{\mathrm{ss}}$, extracted from the data in Fig.~\ref{S3}. The square, two-step, and three-step pulses are shown in blue, red, and green, respectively, while solid, dashed, and dotted curves in every panel correspond to the post-readout total error probability $\widetilde{P}_{\mathrm{err}}^i$, the $n_g$-averaged transition probability $\overline{P^i_{m}}(M_3)$, and the overlap error $\varepsilon_{o}(M_2)$, respectively. Experimental data are shown in (a),(b), with the measured $\overline{P^i_{m}}(M_3)$ for the square, two-step, and three-step pulses marked by dashed curves with circles (blue), squares (red), and triangles (green), respectively. The corresponding simulated data are shown in (c),(d).}
\label{S4}
\end{figure*}

% \newpage
% \nocite{*}
% \bibliography{SM_citation}

\end{document}
